# Supplementary material for: GelTip Tactile Sensor for Dexterous Manipulation in Clutter
Source: arXiv:2112.01834 source file (2021-12-03)
Supplement: Supplementary file 2 [file appendix02.tex]

\begin{frontmatter}
\chapter{Appendix title}%\label{chap:appb}
\end{frontmatter}
